# Supplementary material for: Absence of high pressure ground state re-entrant ferroelectricity in PbTiO$_3$
Source: arXiv:2310.18421 source file (2024-10-31)
Supplement: Supplementary file 1 [file UHP_PbTiO3_SM.pdf]

## Supplemental Material

R. E. Cohen, Muhtar Ahart, and Russell J. Hemley

### Experimental Methods

#### 1. Sample Loading

PbTiO<sub>3</sub> single crystals were grown by a high-temperature flux method. Single crystal and powder (grounded from a single crystal) samples loaded into the separated diamond anvil cells (DAC) [S1]. To maintain a quasi-hydrostatic-pressure environment, neon was used as the pressure medium for all high-pressure study but in one of the x-ray diffraction experiments argon was used as the pressure medium and indicated in the relevant figure caption. In addition, a small piece of ruby was loaded into the DAC for standard ruby fluorescence measurements of the pressure [S2]. Figure S1 shows an image taken at 60 GPa and 300 K for single crystal PTO. Sample shows slightly yellowish colour and is transparent for most of the visible light.

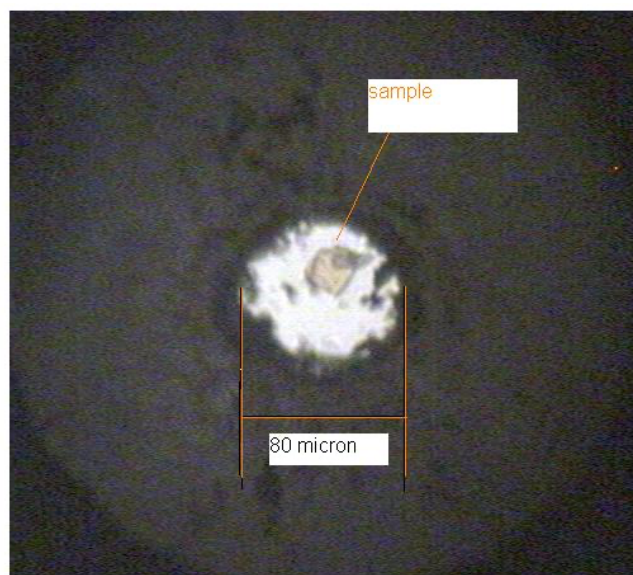

**Figure S1.** Image of PbTiO<sub>3</sub> single crystal in a DAC. Image was taken at 60 GPa and 300 K. The gasket hole size was about 80  $\mu\text{m}$  and sample lateral size was about 30  $\mu\text{m}$ . Neon was used as the pressure transmitting medium.

#### 2. Second Harmonic Generation

The setup for the second harmonic generation (SHG) [S3] measurements is shown in Fig. S2. A near IR (1064  $\mu\text{m}$ ) pulse of a 8-20 ns pulsed laser with a 1-20 kHz repetition rate was used to excite the SHG signal. A dedicated spectrograph equipped with a charge-coupled-device (CCD) detector synchronized with the laser is used for the SHG signal acquisitions [S4]. The acquisition time was about 2s. Measurements were performed at 10 and 300 K. Additional details can be found in Ref. S4.

According to standard Landau theory, the second nonlinear harmonic of the dielectric permittivity is finite only if the crystal symmetry is broken such that the crystal

does not possess a centre of symmetry [S5]. First-principles calculations [S6,S7] predict that  $\text{PbTiO}_3$  should have a ( $I4\text{cm}$ ) polar structure above 40 GPa) resulting in a spontaneous polarization that would induced the SGH signal. However, we did not observe the predicted enhanced SGH signal; rather, the effect remained extremely weak at these pressures, indicating that no polarization exists under these conditions, in contrast to the predictions of Refs. S6 & S7.

The SHG effect is a nonlinear optical effect resulting from a nonlinear dependence of the polarization on the electric field. The linear response connects the polarization at frequency  $\omega$  and the field at the same frequency, and the nonlinear response produces polarization harmonics. For instance, the second harmonic is the polarization at the doubled frequency, the appearance of which results from the product of two components of the field generated at frequency  $\omega$

$$P_i(2\omega) = \varepsilon_0 \chi_{ijk} E_j(\omega) E_k(\omega) , \quad (1)$$

where  $\chi$  is the second-order susceptibility tensor which is non-zero for noncentrosymmetric system only. In ideal ferroelectric crystals, the light is scattered by the set of the uniformly displaced ions. The corresponding peak is as sharp as the x-ray Bragg peak. The theory predicts that the second harmonic couples directly to the symmetry-breaking order-parameter or spontaneous polarization [S5].

In general, the SGH signal is sensitive to the domain structure of ferroelectrics and their orientations<sup>8</sup>. In our high pressure experiments, the selection of polarization of incident or scattering light is restricted, as well as the sensitive of SGH signal to the domain is restrained due to the stressed diamond window. Although the intensity of SGH obtained from single crystal samples shows some fluctuations with pressure within the ferroelectric phase (below 12 GPa), nevertheless, it displays consistence behavior under pressure with that of powder samples (Fig. 3 of main text). Thus, we can consider that we are measuring an averaged total intensity of SGH signal which, in principle, is proportional to the square of averaged spontaneous polarization of the samples<sup>8</sup>:

$$I \propto \langle P_s \rangle^2 \quad (2)$$

where  $P_s$  is the spontaneous polarization. To the contrary, our results exhibit that the possibility of high pressure ferroelectricity in  $\text{PbTiO}_3$  are small in the pressure range up to 100 GPa at least at room temperature. Our x-ray diffraction data show the pressure induced successive phase indeed existing in  $\text{PbTiO}_3$  at room temperature, however, the SGH signal did not couple to these phase transitions indicating the nature of the phase transitions are elastic.

In addition, we also performed the SHG measurements at 10 K up to 60 GPa. The pressure dependence of the intensity of SHG decreases with pressure after 12 GPa and becomes almost zero at 24 GPa (Fig. S3), but no enhancement is observed above this pressure. The phase boundary (24 GPa) is consistent with the previous study (Ref. 5 of main text).

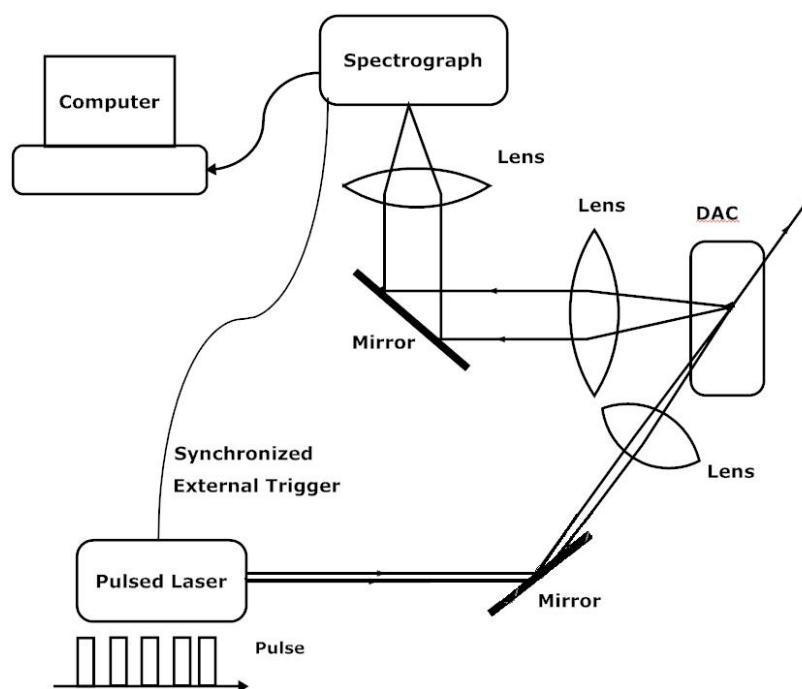

**Figure S2.** Schematic diagram for second harmonic generation (SHG) measurements. A pulsed laser (1064 nm), a spectrograph, and a CCD detector (not shown in the figure but it is the part of spectrograph) were synchronized with the external trigger source. The excitation laser beam from the pulsed laser was guided (by mirror and lenses) into the sample inside of the DAC. Scattered light (SHG signal) was collected by an objective lens, focused into the spectrograph, and detected by a CCD detector. The spectrograph was set to the second harmonic region which was 532 nm (half of the incident light).

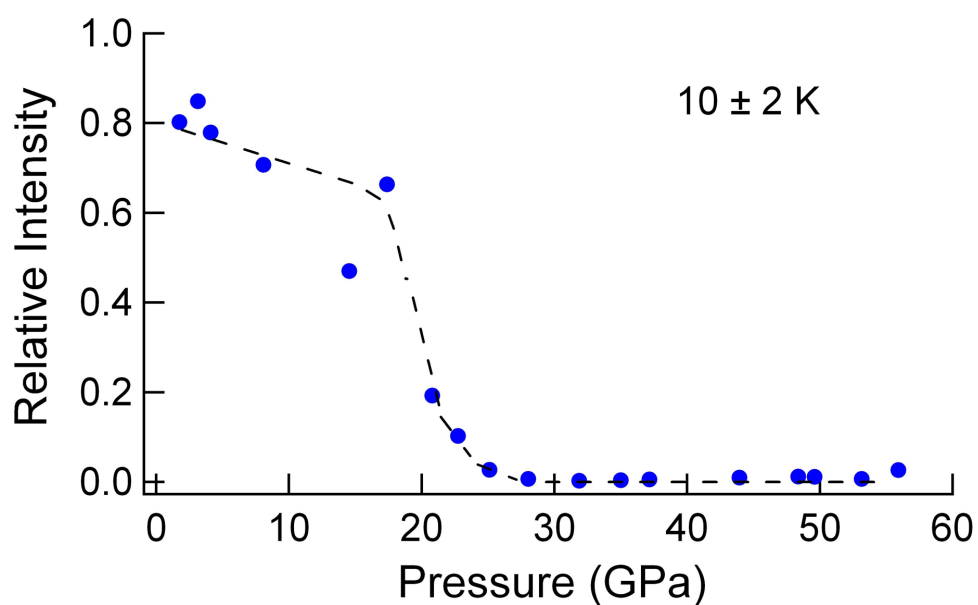

Figure S3. Pressure dependence of intensity of the SHG. The intensity was normalized with the intensity at ambient conditions. No intensity enhancement was observed above 24 GPa.

### 3. Raman Scattering

Figure S4 shows the typical low frequency Raman spectra. These were obtained from a home-built Raman system consisting of a solid state 532 nm laser for excitation, Acton Spectrograph with CCD detector (Princeton Instruments) equipped with the narrow notch filters that allows detection to low frequencies of  $10\text{ cm}^{-1}$ . In order to observe the clear trend of the spectra as a function of pressure, the measured spectra were divided by a white light spectrum in Fig. S4. Figure S5 shows the high frequency Raman spectra (which obtained from a Jobin Yvon HR-460 single grating system combined with the double notch filters with higher throughput, but a higher low frequency cut off of  $80\text{ cm}^{-1}$ ) as a function of pressure at 300 K. In order to clarify the spectra features, the spectra were enlarged 5 times between 12 and 30 GPa; and 10 times above 30 GPa.

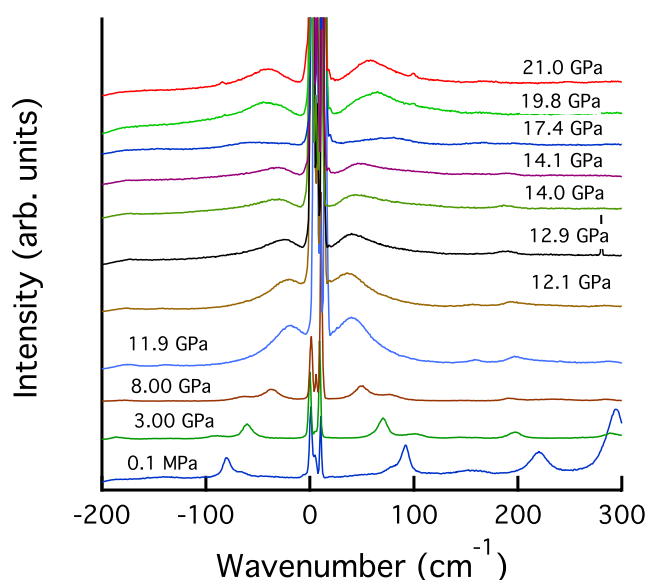

**Figure S4.** Low frequency Raman spectra of  $\text{PbTiO}_3$  at selected pressures at 300 K. Two Raman modes, near  $100\text{ cm}^{-1}$  at ambient pressure, show strong softening toward 12 GPa at 300 K. The Raman mode reappears as a single peak above 12 GPa, but remains rather broad to higher pressures. The intensities for each spectrum were normalized with a white light source.

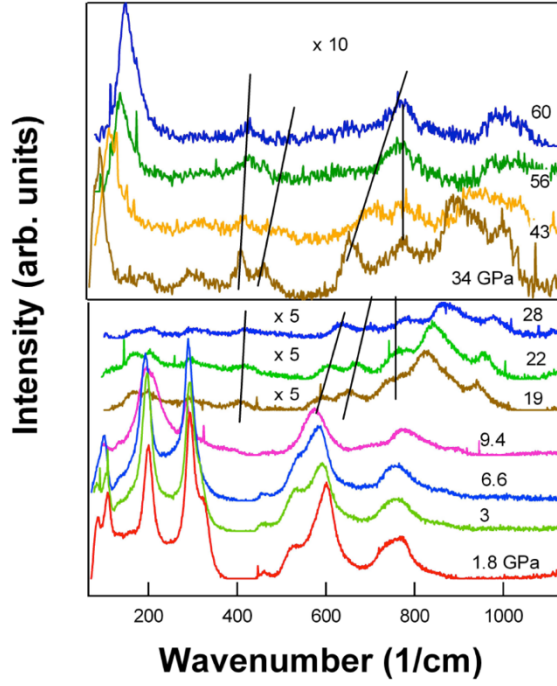

**Figure S5.** High frequency Raman spectra of  $\text{PbTiO}_3$  at selected pressures at 300 K. The spectra correspond to 19, 22, and 28 GPa were enlarged 5 times and indicated by  $\times 5$ ; the spectra correspond to 34, 43, 56, and 60 GPa were enlarged by  $\times 10$ .

Figure S6 shows the comparison of P-dependencies of soft-modes at 10 and 300 K. Two soft modes show softening toward 12 GPa at 300 K, the results are consistent with the previous study [S7]. On the other hand, one of these two soft-modes soften toward the 16 GPa and becomes hard-mode after that at 10 K; and second mode shows softening toward 24 GPa. These behaviours are discussed in details in Ref. 5 of main text.

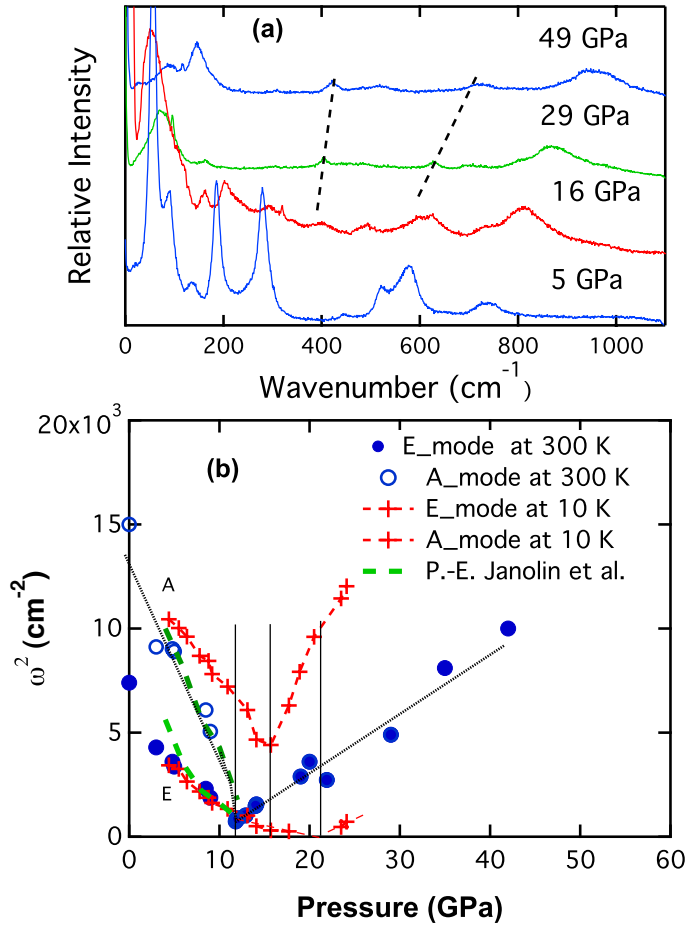

**Figure S6.** Pressure dependencies of the soft modes. Panel (a) shows the spectra at selected pressures at 300 K; panel (b) shows the pressure dependencies of soft-modes. Open and solid circles represent the soft modes measured at 300 K; Cross symbol plus dashed curves represent soft modes at 10 K (Ref. 5); and thick dashed curves represent the soft modes obtained by Janolin et al (Ref. 4). Short-dashed curves are guide for eyes. Inset shows the Raman spectra at selected pressures.

#### 4. X-ray Diffraction

The powder samples of lead titanate were loaded into stainless steel gaskets in a DAC with Ne as the pressure medium. In addition, small ruby chips and Au powder were loaded together with samples for pressure determination. We carried out the angular dispersive x-ray diffraction (ADXRD) experiments at beamline 16-BM-D of HPCAT at the Advanced Photon Source, Argonne National Laboratory. Figures S7 show the obtained diffraction patterns at selected pressures.

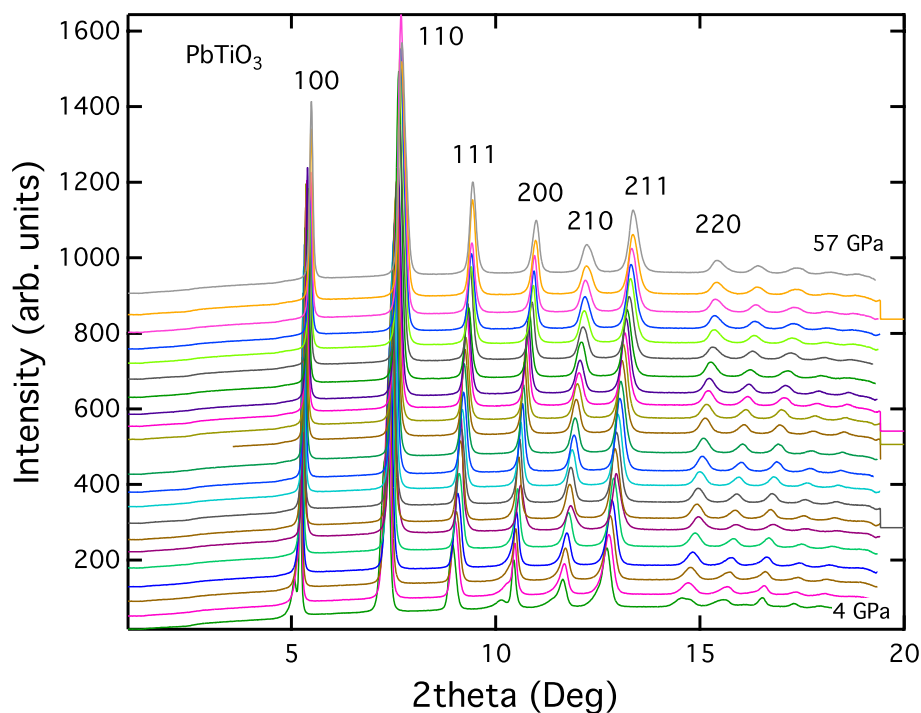

**Figure S7.** X-ray diffraction patterns at selected pressures up to 60 GPa. Neon was used as the pressure transmitting medium. Pseudo-cubic indexing was used to assign each Bragg peak. Perovskite structure is preserved at least up to 60 GPa. Note that the x-ray wavelength (0.354241 Å) differed from that of the experimental results shown in Fig. S7.

## 5. X-ray Diffraction Analysis

We performed the Retveld fitting {GSAS package: A. C. Larson and R. B. Von dreele, General Structure Analysis System, Los Alamos National Laboratory Report LAUR 86-748 (2004)} on collected x-ray diffraction patterns below 30 GPa. We used atomic coordinates in  $P4mm$  space group for the data between ambient and 12 GPa; and  $Pm-3m$  between 12 and 30 GPa. Our results are consistent with the previous studies in the similar pressure ranges. However, we were not able to obtain the best fit of the data above 30 GPa with the following structures:  $Pm-3m$ ,  $R3c$ ,  $R-3c$ ,  $I4cm$ ,  $I4/mcm$ , and  $Pbam$ .

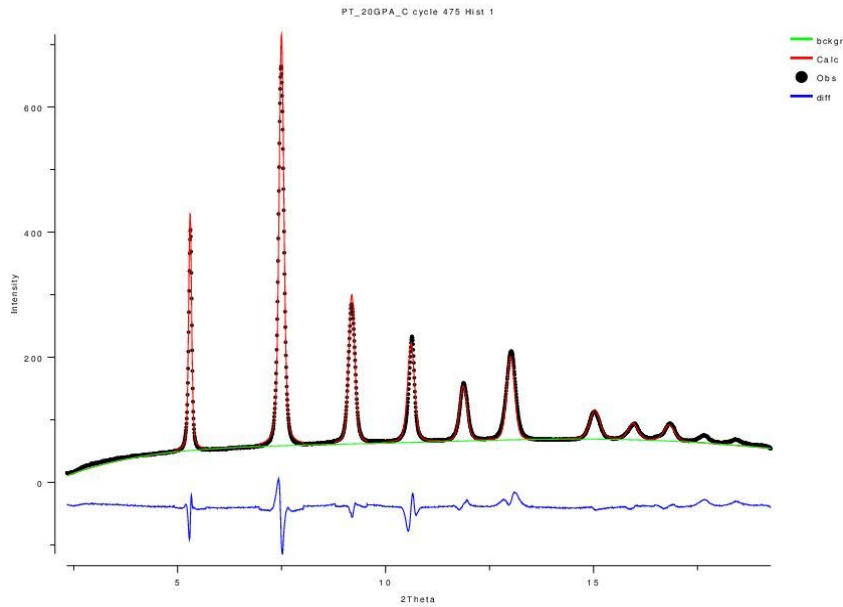

Figure S9. A fitting example using a GSAS Retveld fitting package at 20 GPa. Pseudo-cubic atomic coordinates were used between 12 and 30 GPa; a tetragonal atomic coordinates were used below 12 GPa.

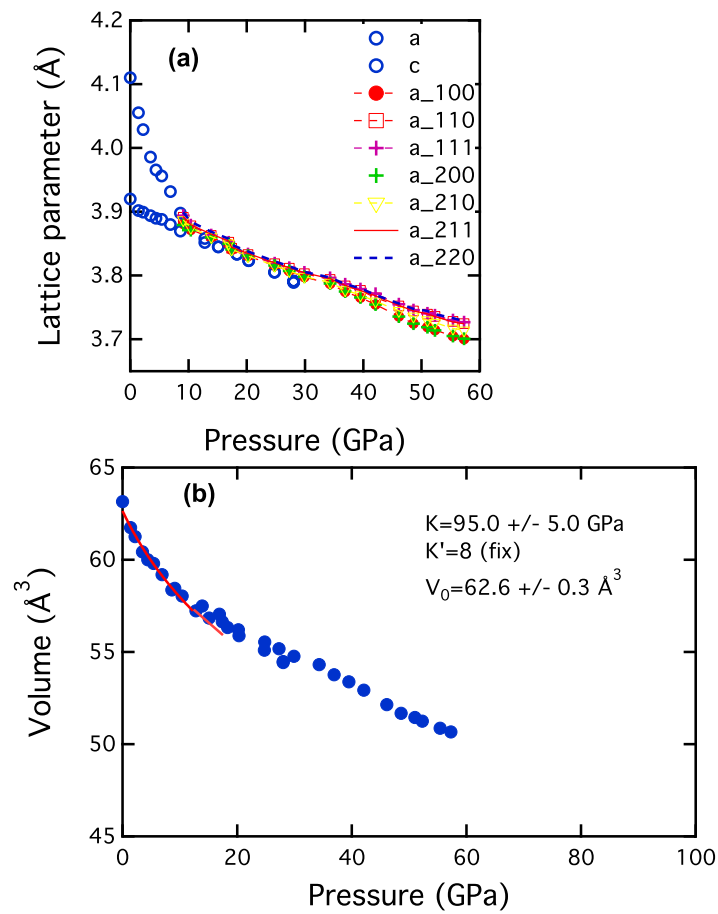

Figure S12. Experimental equation of state. Upper panel (a) shows the pressure dependence of lattice parameters. Note that open circles represent the lattice parameters from fitting; other symbols represent the scaled d-spacing for each Bragg peak (pseudo-cubic indexing) and indicated by solid circles, open squares, solid line, and dashed line, respectively. Lower panel shows the equation of state, Vinet equation of state fit to the data below 12 GPa yields bulk modulus and initial volume, the numerical values are given in the figure.

## References

- [S1] C. E. Weir, E. R. Lipincott, A. V. Valkenburg, and E. N. Bunting, *J. Res. Natl. Bur. Stand.* 63A, 52 (1959).
- [S2] R. A. Forman, G. J. Piermarini, J. D. Barnett, and S. Block, *Science* 176, 284 (1972).
- [S3] V. G. Dmitriev, G. G. Gurzadyan, and D. N. Nikogosyan, *Handbook of Nonlinear Optical Crystals*, (Springer, 1999).
- [S4] A. F. Goncharov, P. Beck, V. V. Struzhkin, R. J. Hemley, and J. C. Crowhurst, *J. Phys. Chem. Solids* 69, 2217 (2008).
- [S5] Y. Ishibashi, *J. Korean Phys. Soc.* 32, S407 (1998).
- [S6] M. Ahart, M. Somayazulu, R. E. Cohen, P. Ganesh, P. Dera, H-k. Mao, R. J. Hemley, R. Yang, P. Liermann, and Z. Wu, *Nature* 451, 545 (2008).
- [S6] I. A. Kornev, L. Bellaiche, P. Bouvier, P.-E. Janolin, and B. Dkhil, J. Kreisel, *Phys. Rev. Lett.* **95**, 196804 (2005).
- [S7] P.-E. Janolin, P. Bouvier, J. Kreisel, P. A. Thomas, I. A. Kornev, L. Bellaiche, W. Crinchton, M. Hanfland, and B. Dkhil, *Phys. Rev. Lett.* 101, 237601 (2008).
- [S8] C. C. Neacsu, B. B. V. Aken, M. Fiebig, and M. B. Raschke, *Phys. Rev. B* 79, 100107 (2009)
